# Supplementary material for: Analysis of Superfast Encoding Performance for Electronic Structure Simulations
Source: arXiv:1907.02976 source file (2020-03-16)
Supplement: Supplementary file 1 [file Appendix1.tex]

\documentclass[main.tex]{subfiles}

\section{Appendix 1: AE6 molecules geometry}

\subsection{Silane}
\begin{lstlisting}
Si   0.0000000    0.0000000    0.0000000
H    0.8124980    0.8124980    0.8124980
H   -0.8124980   -0.8124980    0.8124980
H   -0.8124980    0.8124980   -0.8124980
H    0.8124980   -0.8124980   -0.8124980
\end{lstlisting}
\vspace{10mm}

\subsection{SiO}
\begin{lstlisting}
Si   0.0000000    0.0000000    0.5361840
O    0.0000000    0.0000000   -0.9383220
\end{lstlisting}
\vspace{10mm}

\subsection{Sulfur}
\begin{lstlisting}
S    0.0000000    0.0000000    0.9451780
S    0.0000000    0.0000000   -0.9451780
\end{lstlisting}
\vspace{10mm}

\subsection{Glyoxal}
\begin{lstlisting}
C   -0.3269510    0.6981220    0.0000000
C    0.3269510   -0.6981220    0.0000000
H   -1.4299260    0.6874170    0.0000000
H    1.4299260   -0.6874170    0.0000000
O    0.3269510    1.7270920    0.0000000
O   -0.3269510   -1.7270920    0.0000000
\end{lstlisting}
\vspace{10mm}

\subsection{Propyne}
\begin{lstlisting}
C    0.0000000    0.0000000   -1.2454360
C    0.0000000    0.0000000    0.2386820
C    0.0000000    0.0000000    1.4083610
H    0.0000000    0.0000000    2.4717540
H    0.0000000    1.0191480   -1.6271320
H    0.8826080   -0.5095740   -1.6271320
H   -0.8826080   -0.5095740   -1.6271320
\end{lstlisting}
\vspace{10mm}

\subsection{Cyclobutane}
\begin{lstlisting}
C    0.0000000    1.0969440    0.0386180
C    0.0000000   -1.0969440    0.0386180
C   -1.0969440    0.0000000   -0.0386180
C    1.0969440    0.0000000   -0.0386180
H    0.0000000    1.6442960    0.9772930
H    0.0000000    1.8103180   -0.7810910
H    0.0000000   -1.6442960    0.9772930
H    0.0000000   -1.8103180   -0.7810910
H   -1.6442960    0.0000000   -0.9772930
H   -1.8103180    0.0000000    0.7810910
H    1.6442960    0.0000000   -0.9772930
H    1.8103180    0.0000000   0.7810910]
\end{lstlisting}
\vspace{10mm}
