# Supplementary material for: Analysis of Superfast Encoding Performance for Electronic Structure Simulations
Source: arXiv:1907.02976 source file (2020-03-16)
Supplement: Supplementary file 4 [file AppendixOSEterms.tex]

\begin{table*}
    \centering
    \caption{Second quantized molecular Hamiltonian operators in terms of edge operators in the OSE and the expressions for edge operators in terms of qubit Pauli operators}
    \label{table:OSEterms}
    \begin{tabular}{c c c}
        \hline
        \textbf{Operator type}  & \textbf{Second quantized form} & \textbf{OSE form}\\
        \hline
        Particle creation operator & $a_i^{\dagger}a_j^{\dagger} + a_i a_j $ & $\frac{-i}{2}(A_{ij}B_j - B_i A_{ij} )$ \\[2ex]
        Number operator & $h_{ii}a_i^{\dagger}a_i$  & $\frac{h_{ii}}{2}(1-B_{i})$\\[2ex]
        Coulomb/exchange operator & $h_{ijji}a_i^{\dagger}a_j^{\dagger}a_j a_i $ & $ \frac{h_{ijji}}{4}(1-B_i)(1-B_j)$\\[2ex]
        Excitation operator & $h_{ij}(a_i^{\dagger} a_j +a_j^{\dagger} a_i )$ & $\frac{-i h_{ij}}{2}(A_{ij}B_j + B_i A_{ij}) $\\[2ex]
        Number-excitation operator & $h_{ijjk}(a_i^{\dagger}a_j^{\dagger} a_j a_k + a_k^{\dagger}a_j^{\dagger} a_j a_i) $ & $\frac{-i h_{ijjk}}{4}(A_{ik}B_k + B_i A_{ik})(1-B_j) $\\[2ex]
        Double-excitation operator & $h_{ijkl}(a_i^{\dagger}a_j^{\dagger} a_k a_l + a_l^{\dagger}a_k^{\dagger} a_j a_i)$ & $h_{ijkl} A_{ij} A_{kl}(-1-B_i B_j + B_i B_k+ B_i B_l + B_j B_k$\\
        \qq & \qq & $+ B_j B_i - B_k B_l - B_i B_j B_k B_l)/8$ \\ [2ex]
        \hline
        \textbf{Operator type} & \textbf{OSE operator} & \textbf{Pauli representation}\\[1ex]
        \hline
        Vertex operator & $B_i$ &$\displaystyle \prod_{j: (ij)\in E}\sigma^{z}_{ij}$ \\[2ex]
        Edge operator & $A_{ij}$ & $\epsilon_{ij} \sigma^{x}_{ij}\prod_{l<j}^{n(i)} \sigma^{z}_{li} \prod_{s<j}^{n(j)} \sigma^{z}_{sj}$\\[2ex]
        \hline
    \end{tabular}

\end{table*}
